# Supplementary material for: Dimension Reduction for Efficient Dense Retrieval via Conditional Autoencoder
Source: arXiv:2205.03284 source file (2022-10-22)
Supplement: Supplementary file 1 [file appendix.tex]

\section{Appendix}
